# Supplementary material for: Physical-Variable-Informed Deep Learning for Robust Diagnosis in Industrial Fluid Transport Systems
Source: arXiv:2610.27891 source file (2026-10-20)
Supplement: Supplementary file 1 [file SupportingInformation.tex]

% !TeX program = pdflatex
% Compile this file to generate SupportingInformation.pdf.
\def\SUPPLEMENTARY{1}
\input{sn-article.tex}
